# Supplementary material for: Haskelite: A Tracing Interpreter Based on a Pattern-Matching Calculus
Source: arXiv:2407.11831 source file (2024-07-16)
Supplement: Supplementary file 1 [file appendix.tex]

\section{Proof sketches}

\subsection{Theorem~\ref{thm:soundness1}} \label{app:soundness1}

\paragraph{Theorem}[$\Downarrow$ implies $\Rightarrow^{*}$]
  If
  \[ \Gamma; \lset; e \expev \Delta; w \]
  then for all $S$
  \[ (\Gamma, \eval e,  \retstack) \Rightarrow^{*}
    (\Delta, \eval w, \retstack)
  \]

  If
  \[ \Gamma; \lset; \argstack; m \matev \Delta; \matchresult
  \]
  then for all $S$
  \[
    (\Gamma, \match{\argstack}{m}, \retstack) \Rightarrow^{*}
    (\Delta, \match{[\,]}{\matchresult}, \retstack)
  \]

\begin{proof} The proof is by induction on the height of
  the evaluation derivations of $\expev$ and $\matev$.
  We proceed by analysis on the last rule used.

  \paragraph{Case \bigrule{App}}
  The evaluation rule is
  \[ \prooftree
    \Gamma;\lset; e \expev \Delta;\lambda m \qquad
    \Delta;\lset; \lambda (\matcharg{y}{m}) \expev \Theta; w
    \justifies
    \Gamma;\lset; (e~y) \expev \Theta; w
    \endprooftree
  \]
  Let $S$ be arbitrary and $S' = y:S$; applying the induction hypothesis we get
  \begin{gather*}
    (\Gamma, \eval e, S') \Rightarrow^{*} (\Delta, \eval (\lambda m), S') \\
    (\Delta, \eval \lambda (\matcharg{y}{m}), S) \Rightarrow^{*} (\Theta, \eval e, S)
  \end{gather*}
  Because $\lambda m$ is in whnf we know that $\arity{m}>0$.
  We obtain the proof obligation as follows:
  \[ \begin{split}
    (\Gamma, \eval (e~y), S) &\stackrel{\textsc{App1}}{\Rightarrow}
    (\Gamma, \eval e, y:S) \Rightarrow^{*} (\Delta, \eval (\lambda m), y:S) \\
    & \stackrel{\textsc{App2}}{\Rightarrow} (\Delta, \eval \lambda
    (\matcharg{y}{m}), S) \Rightarrow^{*} (\Theta, \eval e, S)
  \end{split}
\]

\paragraph{Case \bigrule{Sat}}
The evaluation rule is
\[
  \prooftree
  \arity{m}= 0 \qquad
  \Gamma; \lset; [\,];\, m \matev \Delta;\matchreturn{e} \qquad
  \Delta; \lset; e \expev \Theta;\,w
  \justifies
  \Gamma;\lset; \lambda m \expev \Theta;w
  \endprooftree
\]
Let $\retstack$ be arbitrary and $\retstack' = \$:\retstack$; the induction hypotheses give
\begin{gather*}
  (\Gamma, \match{[\,]}{m}, \retstack') \Rightarrow^{*}
  (\Delta, \match{[\,]}{\matchreturn{e}}, \retstack') \\
  (\Delta, \eval e, \retstack) \Rightarrow^{*}
  (\Theta, \eval w, \retstack)
\end{gather*}
We obtain the proof obligation as
\[
  \begin{split}
    (\Gamma, \eval \lambda m, \retstack) & \stackrel{\textsc{Sat}}{\Rightarrow}
    (\Gamma, \match{[\,]}{m}, \$:\retstack) \Rightarrow^{*}
    (\Delta, \match{[\,]}{\matchreturn{e}}, \$:\retstack) \\
    & \stackrel{\textsc{Return1B}}{\Rightarrow}
    (\Delta, \eval{e}, \retstack) \Rightarrow^{*} (\Theta, \eval{w}, \retstack)    
  \end{split}
  \]

  \paragraph{Case \bigrule{Var}}
  The evaluation rule is
  \[
    \prooftree
    \Gamma;\lset\cup\{\loc\}; e \expev \Delta; w 
    \justifies
    \Gamma[\loc\mapsto e]; \lset; \loc \expev \Delta[\loc\mapsto w]; w
    \endprooftree 
  \]
  Let $S$ be arbitrary and $S' = \loc:S$. Applying the induction hypothesis to
  the premise gives
  \[
    (\Gamma, \eval{e}, S') \Rightarrow^{*} (\Delta, \eval{w}, S')
  \]
  We obtain the proof obligation as
  \[
    \begin{split}
      (\Gamma[\loc\mapsto e], \eval{\loc}, S) &
      \stackrel{\textsc{Var}}{\Rightarrow} (\Gamma, \eval{e}, S')  \Rightarrow^{*} (\Delta,\eval{w}, S') \\
      & \stackrel{\textsc{Update}}{\Rightarrow} (\Delta[\loc\mapsto w], \eval{w}, S)
      \end{split}    
  \]
  
  \paragraph{Case \bigrule{Return}}
  The evaluation rule is
  \[
    \prooftree
    \justifies
    \Gamma; \lset; \argstack; \matchreturn{e} \matev \Gamma; \matchreturn{\matcharg{\argstack}{e}}
    \endprooftree     
  \]
  The proof obligation follows by an application of \smallrule{Return1A}:
  \[
  (\Gamma, \match{\argstack}{\matchreturn{e}}, S)
  \stackrel{\textsc{Return1A}}{\Rightarrow}
  (\Gamma, \match{[\,]}{\matchreturn{\matcharg{\argstack}{e}}}, S)
  \]

  \paragraph{Case \bigrule{Fail}}
  The evaluation rule is
  \[
    \prooftree
    \justifies
    \Gamma; \lset; A; \matchfail \matev \Gamma;\matchfail
    \endprooftree
  \]
  The proof obligation follows trivially by either the empty sequence
  (if $A=[\,]$) or an application of \smallrule{Return1C}.
    
  \paragraph{Case \bigrule{Arg}}
  The evaluation rule is
  \[
    \prooftree
    \Gamma; \lset; (y:\argstack); m \matev \Delta;\matchresult
    \justifies
    \Gamma; \lset; \argstack; \matcharg{y}{m} \matev \Delta; \matchresult
    \endprooftree    
  \]
  The induction hypothesis gives
  \[
    (\Gamma, \match{(y:\argstack)}{m}, \retstack) \Rightarrow^{*}
    (\Delta, \match{[\,]}{\matchresult}, \retstack) 
  \]
  Using \smallrule{Arg} gives the required proof obligation:
  \[ 
      (\Gamma, \match{\argstack}{(\matcharg{y}{m})}, \retstack)
      \stackrel{\textsc{Arg}}{\Rightarrow}
      (\Gamma, \match{(y:\argstack)}{m}, \retstack)
      \Rightarrow^{*} (\Delta, \match{[\,]}{\matchresult}, \retstack)    
    \]

    \paragraph{Case \bigrule{Alt1}}
    The evaluation rule is
    \[
    \prooftree
    \Gamma;\lset;\argstack; m_1 \matev \Delta;\matchreturn{e}
    \justifies
    \Gamma;\lset;\argstack; (\matchalt{m_1}{m_2}) \matev \Delta;\matchreturn{e}
    \endprooftree       
  \]
  Let $S$ be arbitrary and $S' = (?(A,m_2)):S$. Applying the induction hypothesis gives
  \[
    (\Gamma, \match{\argstack}{m_1}, S') \Rightarrow^{*}
    (\Delta, \match{[\,]}{\matchreturn{e}}, S')
  \]
  The proof obligation is
  \[
    \begin{split}
      (\Gamma, \match{\argstack}{(\matchalt{m_1}{m_2})}, S) &
      \stackrel{\textsc{Alt1}}{\Rightarrow}
      (\Gamma, \match{\argstack}{m_1}, S') \Rightarrow^{*}
      (\Delta, \match{[\,]}{\matchreturn{e}}, S') \\
      & \stackrel{\textsc{Return2}}{\Rightarrow}
      (\Delta, \match{[\,]}{\matchreturn{e}}, S)
    \end{split}
  \]

  \paragraph{Case \bigrule{Alt2}}
  The evaluation rule is
  \[
    \prooftree
    \Gamma;\lset;\argstack; m_1 \matev \Delta;\matchfail  \qquad
    \Delta;\lset;\argstack; m_2 \matev \Theta; \matchresult
    \justifies
    \Gamma;\lset;\argstack; (\matchalt{m_1}{m_2}) \matev \Theta;\matchresult
    \endprooftree
  \]
  Let $S$ be arbitrary and $S' = (?(\argstack,m_2)):S$. The induction hypothesis gives
  \begin{gather*}
    (\Gamma, \match{\argstack}{m_1}, S') \Rightarrow^{*}
    (\Delta, \match{[\,]}{\matchfail}, S') \\
    (\Delta, \match{\argstack}{m_2}, S) \Rightarrow^{*}
    (\Theta, \match{[\,]}{\matchresult}, S)
  \end{gather*}
  We can obtain the proof obligation as follows:
  \[
    \begin{split}
      (\Gamma, \match{\argstack}{(\matchalt{m_1}{m_2})}, S)
      & \stackrel{\textsc{Alt1}}{\Rightarrow}
      (\Gamma, \match{\argstack}{m_1}, S')
      \Rightarrow^{*} (\Delta, \match{[\,]}{\matchfail}, S') \\
      & \stackrel{\textsc{Alt2}}{\Rightarrow}
      (\Delta, \match{\argstack}{m_2}, S) \Rightarrow^{*}
      (\Theta, \match{[\,]}{\matchresult}, S)
      \end{split}
  \]
  \end{proof}

  \subsection{Theorem~\ref{thm:soundness2}}\label{app:soundness2}

    \begin{definition}
    A sequence of evaluation steps
    $(\Gamma,C,\retstack) \Rightarrow^{*}
    (\Delta,C',\retstack)$ is \emph{balanced} if
    the initial and final stacks are identical and every intermediate
    stack is of the form $S' = \kont_1:\kont_2:\ldots:\kont_n:S$, i.e.\@
    an extension of the initial stack.
  \end{definition}

  \begin{definition}
    The \emph{trace} of a sequence of small-step evaluation
    steps $(\Gamma,C,\retstack) \Rightarrow^{*}
    (\Delta,C',\retstack')$ is the sequence of rules used in the evaluation.
  \end{definition}

  Consider now the traces $B$ of balanced expression evaluations
  $(\Gamma,\eval{e},\retstack)\Rightarrow^{*}(\Delta,\eval{\whnf},\retstack)$
  and $B'$ for balanced matching evaluations
  $(\Gamma,\match{\argstack}{m},\retstack)\Rightarrow^{*}(\Delta,\match{[\,]}{\matchresult},\retstack)$. Since
  specific rules introduce and eliminate stack continuations, we can
  see by inspection of Figures~\ref{fig:smallstep-1} and~\ref{fig:smallstep-2} that such traces
  must be generated by the following grammars:
\begin{align}
  B &::= \textsc{App1}~ B~ \textsc{App2}~B ~\mid~
      \textsc{Sat}~B'~ \textsc{Return1B}~B
      ~\mid~ \textsc{Var}~B ~ \textsc{Update} ~\mid~ \varepsilon  \label{eq:bal-expr}\\
  B' &::= \textsc{Alt1}~B'~\textsc{Alt2}~B' ~\mid~
       \textsc{Alt1}~B'~\textsc{Return2} \notag \\
    &~\mid~ \textsc{Cons1}~ B ~\textsc{Cons2}~B' ~\mid~
      \textsc{Cons1}~ B~ \textsc{Fail} \notag \\
       &~\mid~ \textsc{Arg}~ B' ~\mid~ \textsc{Bind}~B' 
         ~\mid~ \textsc{Return1A}~B' ~\mid~ \textsc{Return1C}~B' \notag \\ 
 & ~\mid~ \textsc{Where}~B' ~\mid~ \varepsilon
      \label{eq:bal-matching}
\end{align}

The last step before we can state the second soundness result is
to see that we can recover the set $\lset$ of locations under evaluation
used in the big-step semantics from the return stack of the small-step
semantics.
\begin{definition}
  Let $\upd{\retstack}$
  be the set of locations marked
  for updates in a stack \retstack, i.e.\@
  $\upd{\retstack} = \{ y ~:~ (!y) \in \retstack \}$.
\end{definition}

\paragraph{Theorem}[$\Rightarrow^*$ implies $\Downarrow$]
  If $(\Gamma, \eval{e}, \retstack) \Rightarrow^{*} (\Delta, \eval{\whnf},
  \retstack)$ is a balanced expression evaluation then
  $\Gamma;\upd{\retstack}; e \expev \Delta; w$.

  If $(\Gamma, \match{A}{m}, \retstack) \Rightarrow^{*} (\Delta,
  \match{[\,]}{\matchresult}, \retstack)$ is a balanced matching evaluation then
  $\Gamma;\upd{\retstack}; A;m \matev \Delta;\matchresult$

  \begin{proof}
  The proof is by induction on the derivation of balanced evaluations
  following the grammar \eqref{eq:bal-expr} and
  \eqref{eq:bal-matching}.  Each production of the grammar corresponds
  to one big-step evaluation rule for $\expev$ or $\matev$.

  The base case corresponds to empty balanced evaluations;
  the start configurations can only of three forms:
  \begin{description}
  \item[$(\Gamma, \eval{w}, \retstack)$:]
    the proof obligation is given by rule \bigrule{Whnf}.
  \item [$(\Gamma, \match{[\,]}{\matchreturn{e}}, \retstack)$:]
    the proof obligation is given by rule \bigrule{Return}.
  \item [$(\Gamma, \match{[\,]}{\matchfail}, \retstack)$]
    the proof obligation is given by rule \bigrule{Fail}.
  \end{description}

  The remaining cases are non-empty balanced evaluations; we present
  some cases in detail.
  
  \paragraph{Case $\textsc{App1}~B~\textsc{App2}~B$}
  The balanced evaluation must be
  \[
    \begin{split}
      (\Gamma,\eval{(e~y)}, \retstack) & \stackrel{\textsc{App1}}{\Rightarrow}
      (\Gamma, \eval{e}, y:\retstack) \Rightarrow^{*}
      (\Gamma', \eval{(\lambda m)}, y:\retstack) \\
      & \stackrel{\textsc{App2}}{\Rightarrow}
      (\Gamma', \eval{\lambda (\matcharg{y}{m})}, \retstack)
      \Rightarrow^{*} (\Delta, \eval{w}, \retstack)
    \end{split}
  \]
  Applying the induction hypothesis to the evaluation sequences above we get
  \begin{gather*}
    \Gamma;\upd{\retstack};e \expev \Gamma'; \lambda m \\
    \Gamma';\upd{\retstack};\lambda(\matcharg{y}{m}) \expev \Delta;w
  \end{gather*}
  Applying rule \bigrule{App} yields the proof obligation
  $\Gamma;\upd{\retstack};(e~y); \expev \Delta; w$.

  \paragraph{Case $\textsc{Sat}~B'~\textsc{Return1B}~B$}
  The balanced evaluation must be
  \[
    \begin{split}
      (\Gamma, \eval{\lambda m}, \retstack) & \stackrel{\textsc{Sat}}{\Rightarrow}
      (\Gamma, \match{[\,]}{m}, \$:\retstack) \Rightarrow^{*}
      (\Gamma', \match{[\,]}{\matchreturn{e}}, \$:\retstack) \\
      & \stackrel{\textsc{Return1B}}{\Rightarrow}
      (\Gamma', \eval{e}, \retstack) \Rightarrow^{*}
      (\Delta, \eval{w}, \retstack)
    \end{split}
  \]
  Note that $\upd{(\$:\retstack)} = \upd{\retstack}$.
  Applying the induction hypothesis to the evaluation sequences above we get
  \begin{gather*}
    \Gamma;\upd{\retstack}; [\,]; m \matev \Gamma'; \matchreturn{e} \\
    \Gamma';\upd{\retstack}; e \expev \Delta; w
  \end{gather*}
  Applying rule \bigrule{Sat} yields the proof obligation.

  \paragraph{Case $\textsc{Alt1}~B'~\textsc{Alt2}~B'$}
  The balanced evaluation must be
  \[ \begin{split}
      (\Gamma, \match{A}{(\matchalt{m_1}{m_2})}, S) &
      \stackrel{\textsc{Alt1}}{\Rightarrow}
      (\Gamma, \match{A}{m_1}, S') \Rightarrow^{*}
      (\Gamma' \match{[\,]}{\matchfail}, S') \\
      & \stackrel{\textsc{Alt2}}{\Rightarrow}
    (\Gamma', \match{A}{m_2}, S) \Rightarrow^{*}
    (\Delta, \match{[\,]}{\matchresult}, S)
      \end{split}
  \]
  where $S' = @(A,m_2):S$.  Note that $\upd{S'} = \upd{S}$. Applying
  the induction hypothesis to the balanced evaluations above we get
  \begin{gather*}
    \Gamma;\upd{S};A;m_1 \matev \Gamma'; \matchfail \\
    \Gamma';\upd{S};A;m_2 \matev \Delta; \matchresult
  \end{gather*}
  Applying rule \bigrule{Alt2} yields the proof obligation.
\end{proof}

%%% Local Variables:
%%% mode: latex
%%% TeX-master: "main"
%%% End:
